# Supplementary material for: Localized Region Contrast for Enhancing Self-Supervised Learning in Medical Image Segmentation
Source: arXiv:2304.03406 source file (2023-04-06)

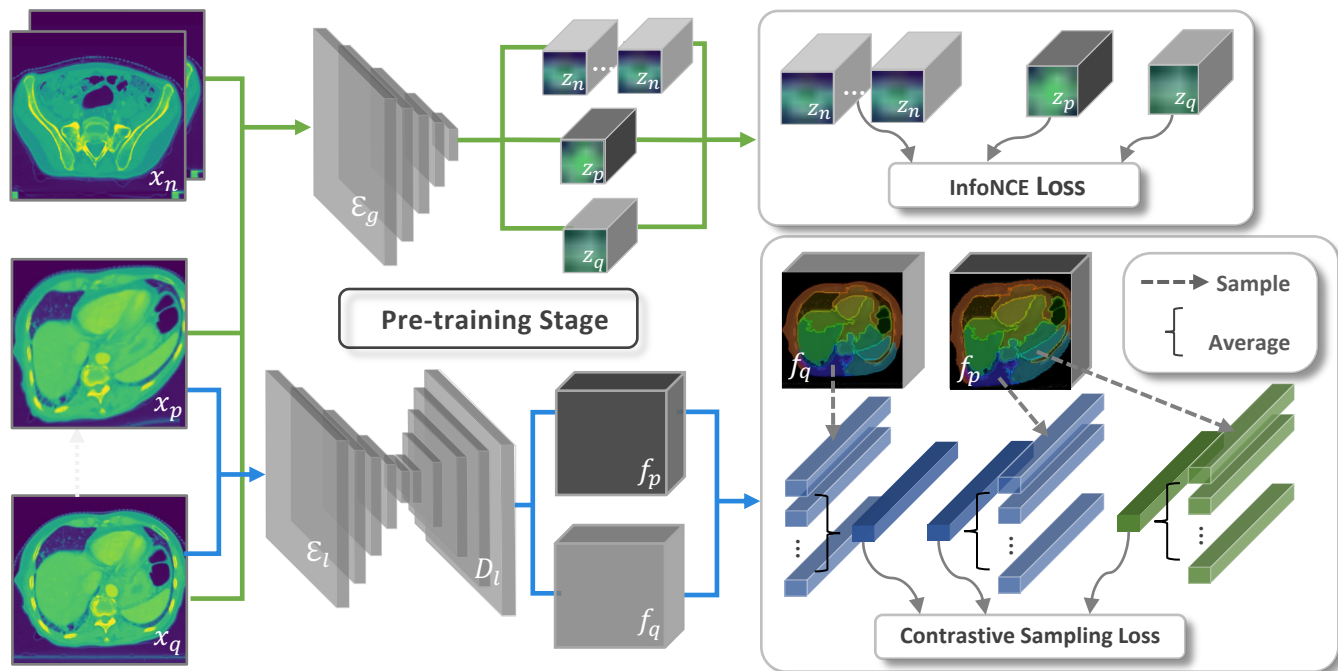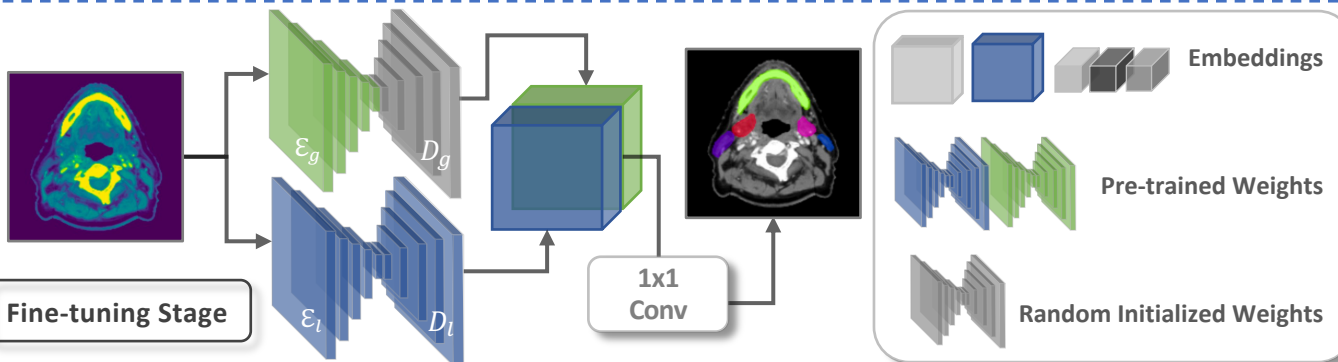

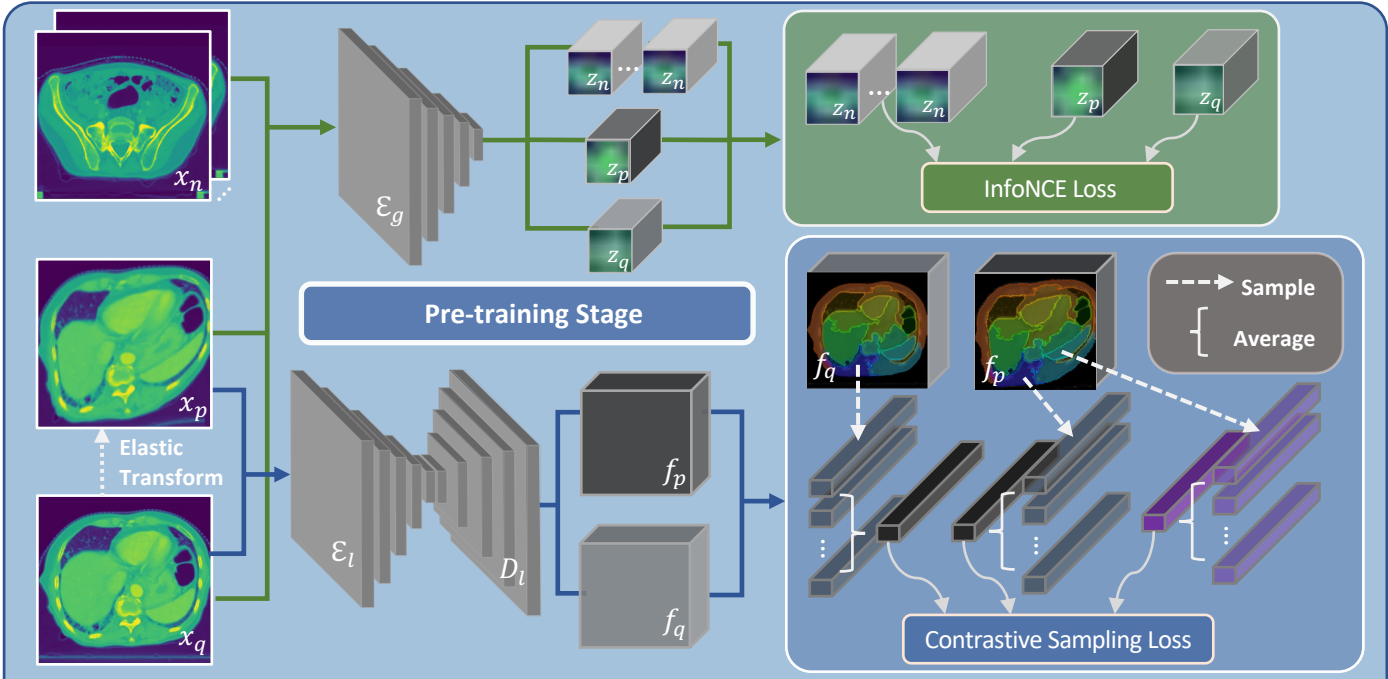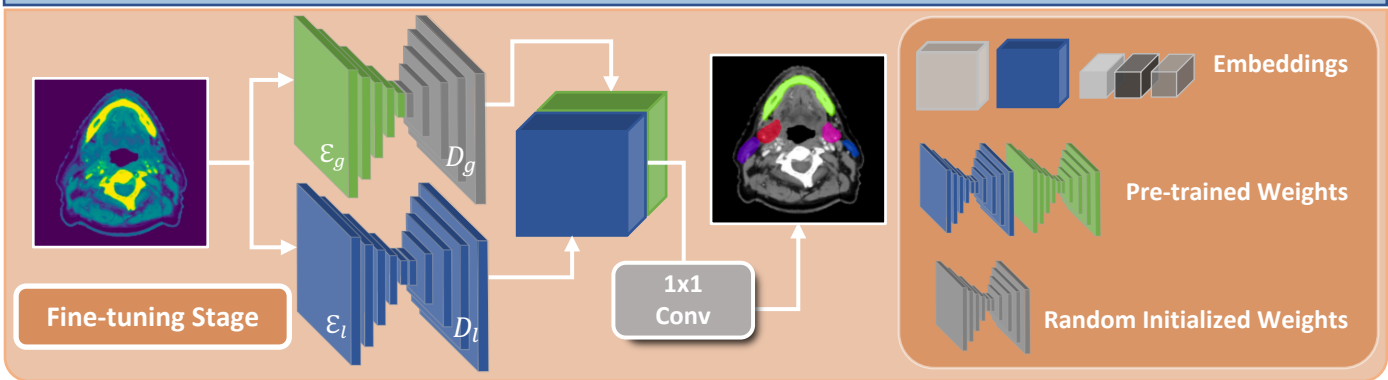

Supplement: Supplementary file 1 [file suppix.pdf]
